# Supplementary material for: CAMixerSR: Only Details Need More "Attention"
Source: arXiv:2402.19289 source file (2024-03-15)
Supplement: Supplementary file 1 [file X_suppl.tex]

\clearpage
\setcounter{page}{1}
% \maketitlesupplementary

\twocolumn[{% 
\renewcommand\twocolumn[1][]{#1}%
\maketitlesupplementary
\begin{center} 
\centering 
\includegraphics[width=1.0\linewidth]{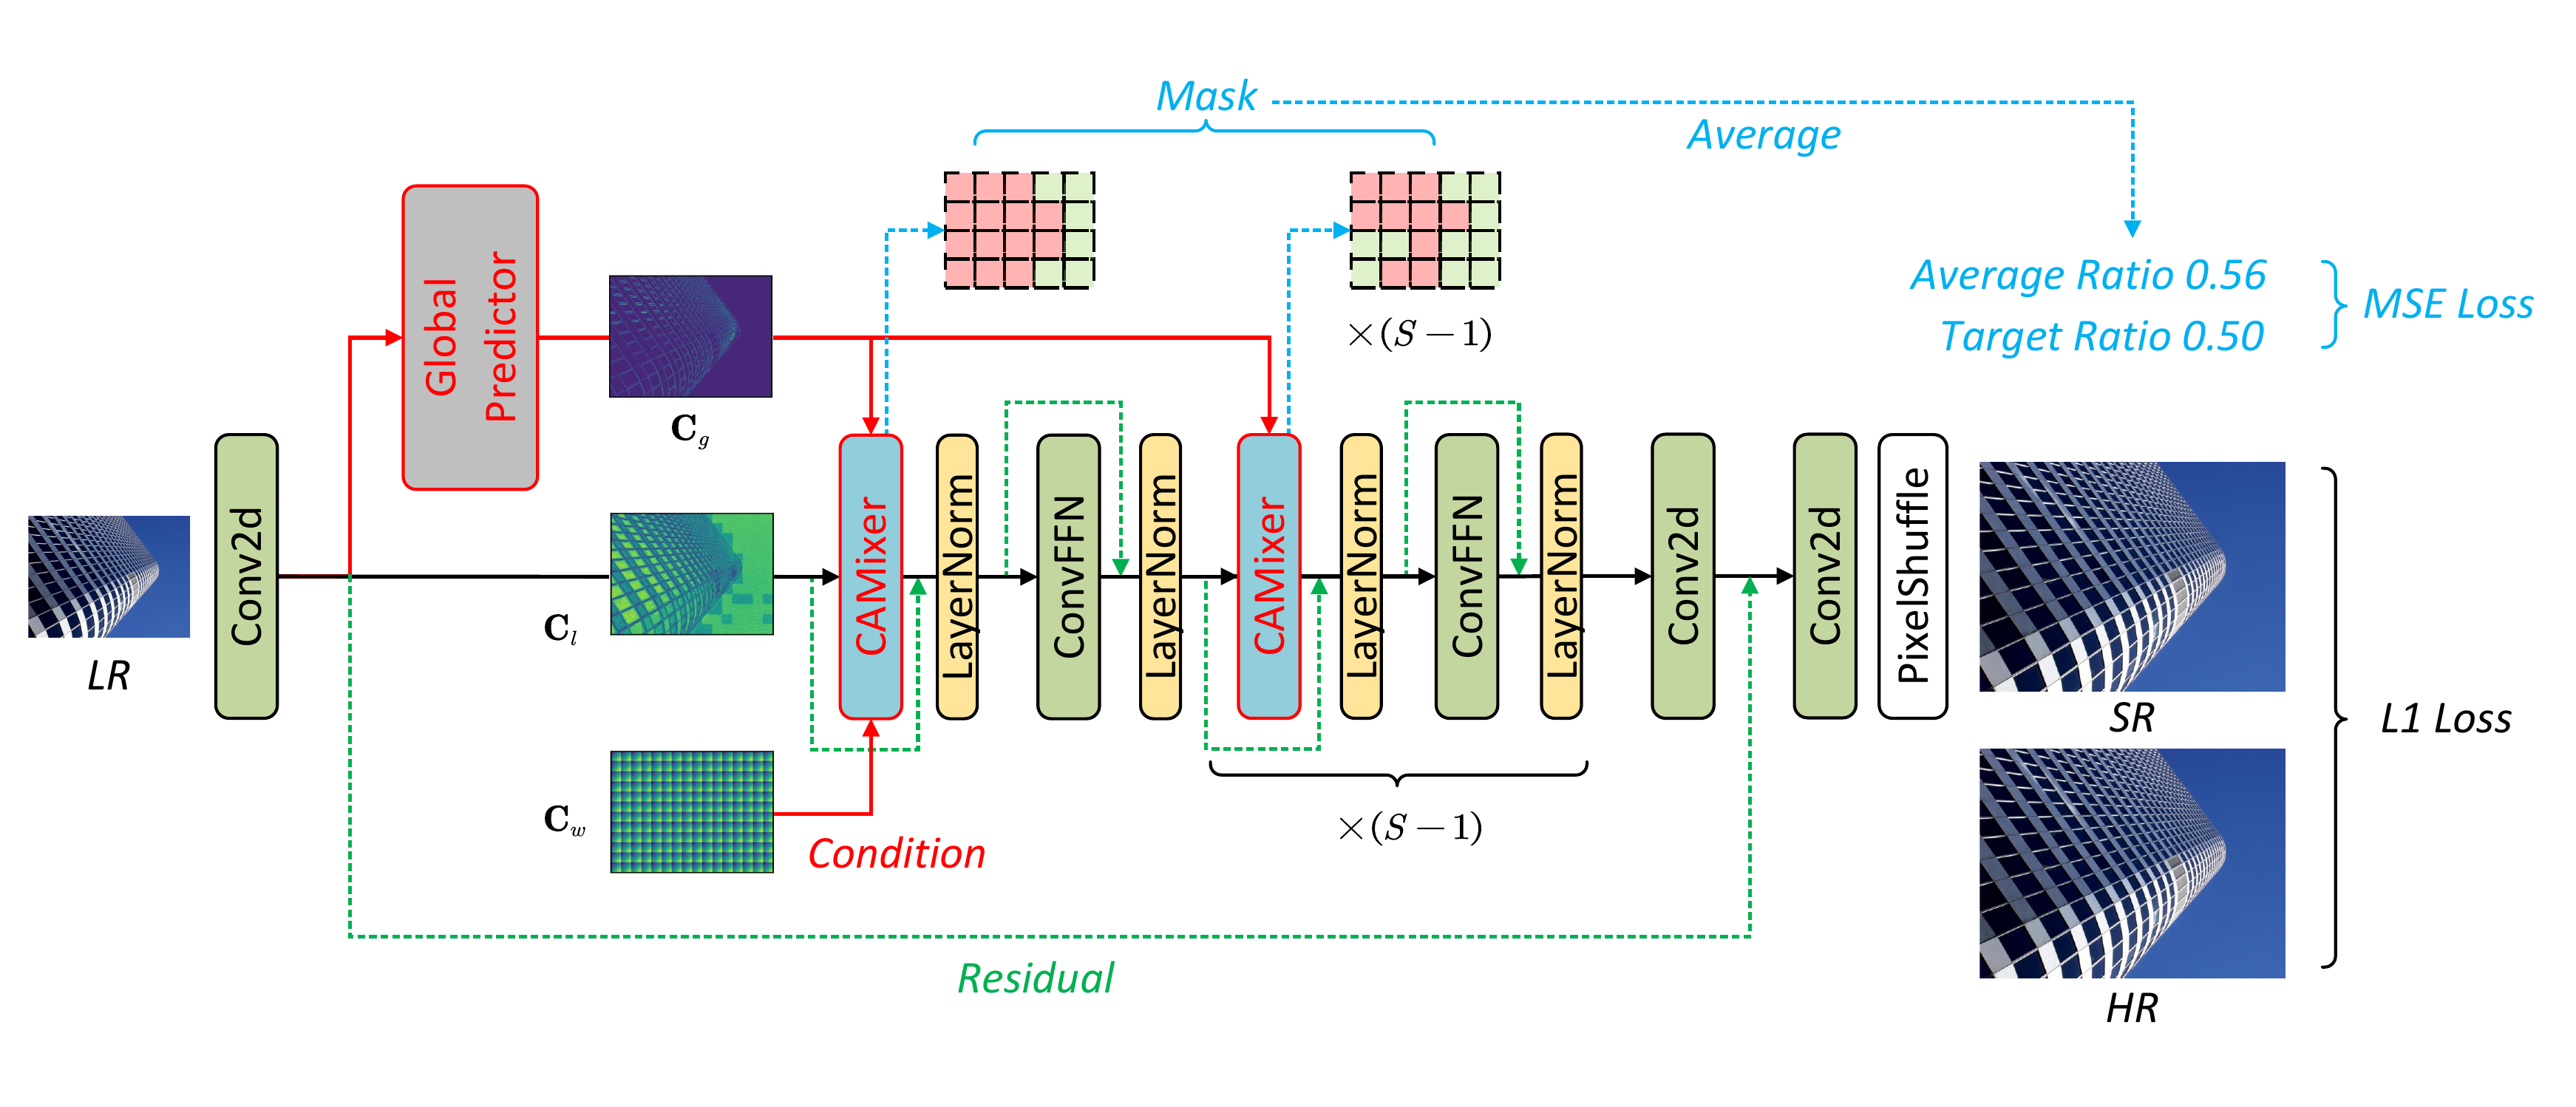}
\captionof{figure}{{Overview of the proposed CAMixerSR framework.} The network architecture is based on SwinIR-light~\cite{SwinIR} but replaces the window-based self-attention with the proposed CAMixer and adds an extra global predictor. (The CAMixer is stacked by group, omitted here for simplicity.) The training framework utilizes two losses, the common $\ell_1$ loss for image restoration and MSE loss for predictor.} 
\label{fig:start2}
\end{center}}]

\section{More Implementation Details}

\subsection{Network Architecture}
We visualize the overall framework of the proposed CAMixerSR in~\cref{fig:start2}. As discussed in the main paper, the CAMixerSR is a modified SwinIR-light~\cite{SwinIR} that uses CAMixer and a global predictor. In general, the CAMixerSR consists of four parts: shallow extractor, deep extractor, reconstruction module, and additional global predictor.

\noindent\textbf{Shallow Extractor (SE)}. Following previous work~\cite{ELAN,EDSR}, given the input low-resolution (LR) image $\rmI_{\etens{LR}}\in\mathbb{R}^{3\times H\times W}$, we employ a 3$\times$3 convolution as the shallow extractor to obtain the initial feature:
\begin{equation}
    \rmF_0 = f_{\etens{Conv}}(\rmI_{\etens{LR}})\in \mathbb{R}^{C\times H\times W}.
\end{equation}

\noindent\textbf{Global Predictor (GP)}. Based on the $\rmF_0$, we employ a global predictor to generate global condition $\rmC_{g}$, which is illustrated in the main paper and stacked by two vanilla convolutions. 
\begin{equation}
    \rmC_{g} = f_{\etens{Global}}(\rmF_{0})\in \mathbb{R}^{2\times H\times W}.
\end{equation}

\noindent\textbf{Deep Extractor (DE)}. Similar to SwinIR~\cite{SwinIR}, we stack the proposed CAMixers and Convolutional Feed-Forward Network (ConvFFN) to accomplish deep feature extraction. Specifically, our DE utilizes the Swinv2~\cite{Swinv2} design for the basic block $f_\etens{Block}$. Given the input feature $\rmF$ and corresponding condition maps $\rmC_g$ and $\rmC_w$, this process can be expressed by:  
\begin{equation}
    \begin{aligned}
        \rmF &= f_\etens{LN}(f_{\etens{CAMixer}}(\rmF,\rmC_g, \rmC_w)+ \rmF), \\ 
        \rmF &= f_\etens{LN}(f_{\etens{FFN}}(\rmF) + \rmF),
    \end{aligned}
\end{equation}
where $f_\etens{LN}(\cdot)$ represents layer normalization. $f_{\etens{CAMixer}}(\cdot)$ and $f_{\etens{FFN}}(\cdot)$ are CAMixer and ConvFFN, respectively.

Then, we stacks total $S$ blocks by group $G$=\{4,4,6,6\} to capture the immediate feature $\rmF_i$, which is formulated by:
\begin{equation}
    \rmF_i = \left\{
    \begin{aligned}
       & f_{\etens{Block}i}(\rmF_{i-1}), \\
       & f_{\etens{Conv}j}(f_{\etens{Block}i}(\rmF_{i-1})) + \rmF_{i-G_j}, 
    \end{aligned}
    \right. i=1,2,...,S 
\end{equation}
where the bottom equation comes into force when it is the tail of the group, \ie, $i$=\{4,10,14,20\}.

\noindent\textbf{Reconstruction Module (RM)}. Following SwinIR-light, we adopt the simplest uscale module to reconstruct the super-resolution image from the captured deep feature:
\begin{equation}
    \rmI_\etens{SR} = f_\etens{RM}(\rmF_S + \rmF_0)\in \mathbb{R}^{3\times sH\times sW},
\end{equation}
where $f_\etens{RM}(\cdot)$ is implemented by a 3$\times$3 convolution to squeeze the channel number $C$ to $3s^2$, and a pixel shuffle operator to transfer depth to space. $s$ indicates the upscale factor.

\begin{algorithm}
\fontsize{8.5pt}{9.5pt}\selectfont
\caption{Training/Inference of CAMixer}\label{algorithm}
\KwData{feature $\rmX$, global condition $\rmC_g$, window condition $\rmC_w$}
\KwResult{refined feature $\rmY$}
calculate the \emph{value}: $\rmV=\rmC_l=f_\etens{PWConv}(\rmX)$\;
\textbf{Predictor}: use conditions ($\rmC_l$, $\rmC_g$, $\rmC_w$) to calculate metrics (mask $m$, offsets $\Delta p$, attentions $\rmA_c$ and $\rmA_s$) based on Eq. {\color{red}2} of main paper\;
calculate warped feature $\Tilde{\rmX}$ by using offsets $\Delta p$ and bilinear interpolation $\phi(\cdot)$:

\eIf{training}{modulate mask by \emph{gumble\_softmax} function~\cite{DynamicViT}: 
$\rmM=\etens{gumble\_softmax}(m)$\;
hard tokens: $\Tilde{\rmX}_\etens{hard} = \Tilde{\rmX}\cdot\rmM$, $\rmV_\etens{hard} =\rmV\cdot\rmM$\;
simple tokens: $\rmV_\etens{simple} =\rmV\cdot(1-\rmM)$\;}
{calculate $K$ by $\sum\rmM$\;
obtain index by \emph{argsort} function: $I=\etens{argsort}(m)$, $I_\etens{hard}=I[:K]$, $I_\etens{simple}=I[K:]$\;
hard tokens: $\Tilde{\rmX}_\etens{hard} = \Tilde{\rmX}[I_\etens{hard}]$, $\rmV_\etens{hard} = \rmV[I_\etens{hard}]$\;
simple tokens: $\rmV_\etens{simple} = \rmV[I_\etens{simple}]$\;}
 
calculate \emph{query} and \emph{key} by: $\Tilde{\rmQ}=\Tilde{\rmX}_\etens{hard}\rmW_q$,  $\Tilde{\rmK}=\Tilde{\rmX}_\etens{hard}\rmW_k$\;
\textbf{Attention}: use self-attention for complex areas: $    {\rmV}_{\etens{hard}} = \etens{softmax}(\frac{\Tilde{\rmQ}\Tilde{\rmK}^{T}}{\sqrt{d}}){\rmV}_{\etens{hard}}$\;
use convolutional sptial attention for simple areas:
${\rmV}_{\etens{simple}} = {\rmV}_{\etens{simple}}\cdot\rmA_s$\;

\eIf{training}
{${\rmV}_{\etens{attn}}={\rmV}_{\etens{hard}}+{\rmV}_{\etens{simple}}$\;}
{${\rmV}_{\etens{attn}}[I_\etens{hard}]={\rmV}_{\etens{hard}}$, ${\rmV}_{\etens{attn}}[I_\etens{simple}]={\rmV}_{\etens{simple}}$\;}

\textbf{Convolution}: calculate convolution and channel attention: ${\rmV}_{\etens{conv}} = f_{\etens{DWConv}}({\rmV}_{\etens{attn}})\cdot\rmA_c + {\rmV}_{\etens{conv}}$\;

project to obtain output $\rmY=f_\etens{PWConv}({\rmV}_{\etens{attn}})$.
\end{algorithm}

\subsection{Training and Inference of CAMixer}
For the proposed CAMixer, we utilize two implementations for training and inference as shown in~\cref{algorithm}.

\noindent\textbf{Inference}. For inference, as formulated in the main paper (Eq.~{\color{red}{4}}), we use the \emph{argsort} to obtain the indices, and then select the top-$K$ tokens to calculate the self-attention. Despite directness and simplicity, this process is non-differentiable.  

\noindent\textbf{Training}. Following DynamicViT~\cite{DynamicViT}, we leverage \emph{gumble\_softmax} function to generate differentiable 0-1 mask $\rmM$ for training, where the index “1” represents the mask of the tokens processed by self-attention. Moreover, \emph{gumble\_softmax} function generates one-hot tensor, of which the expectation equals $m$ exactly.
Specifically, to enable the dynamical adjustment of the attention ratio $\gamma$, the dimension of the softmax is 1 rather than 0 for $m'\in\mathbb{R}^{\frac{HW}{M^2}\times 2}$, where $m'$ is the original output from the predictor.

\begin{figure}
\fontsize{8.5pt}{9.5pt}\selectfont
\tabcolsep=1pt
    \centering
    \begin{tabular}{cr}
             \includegraphics[width=0.48\linewidth]{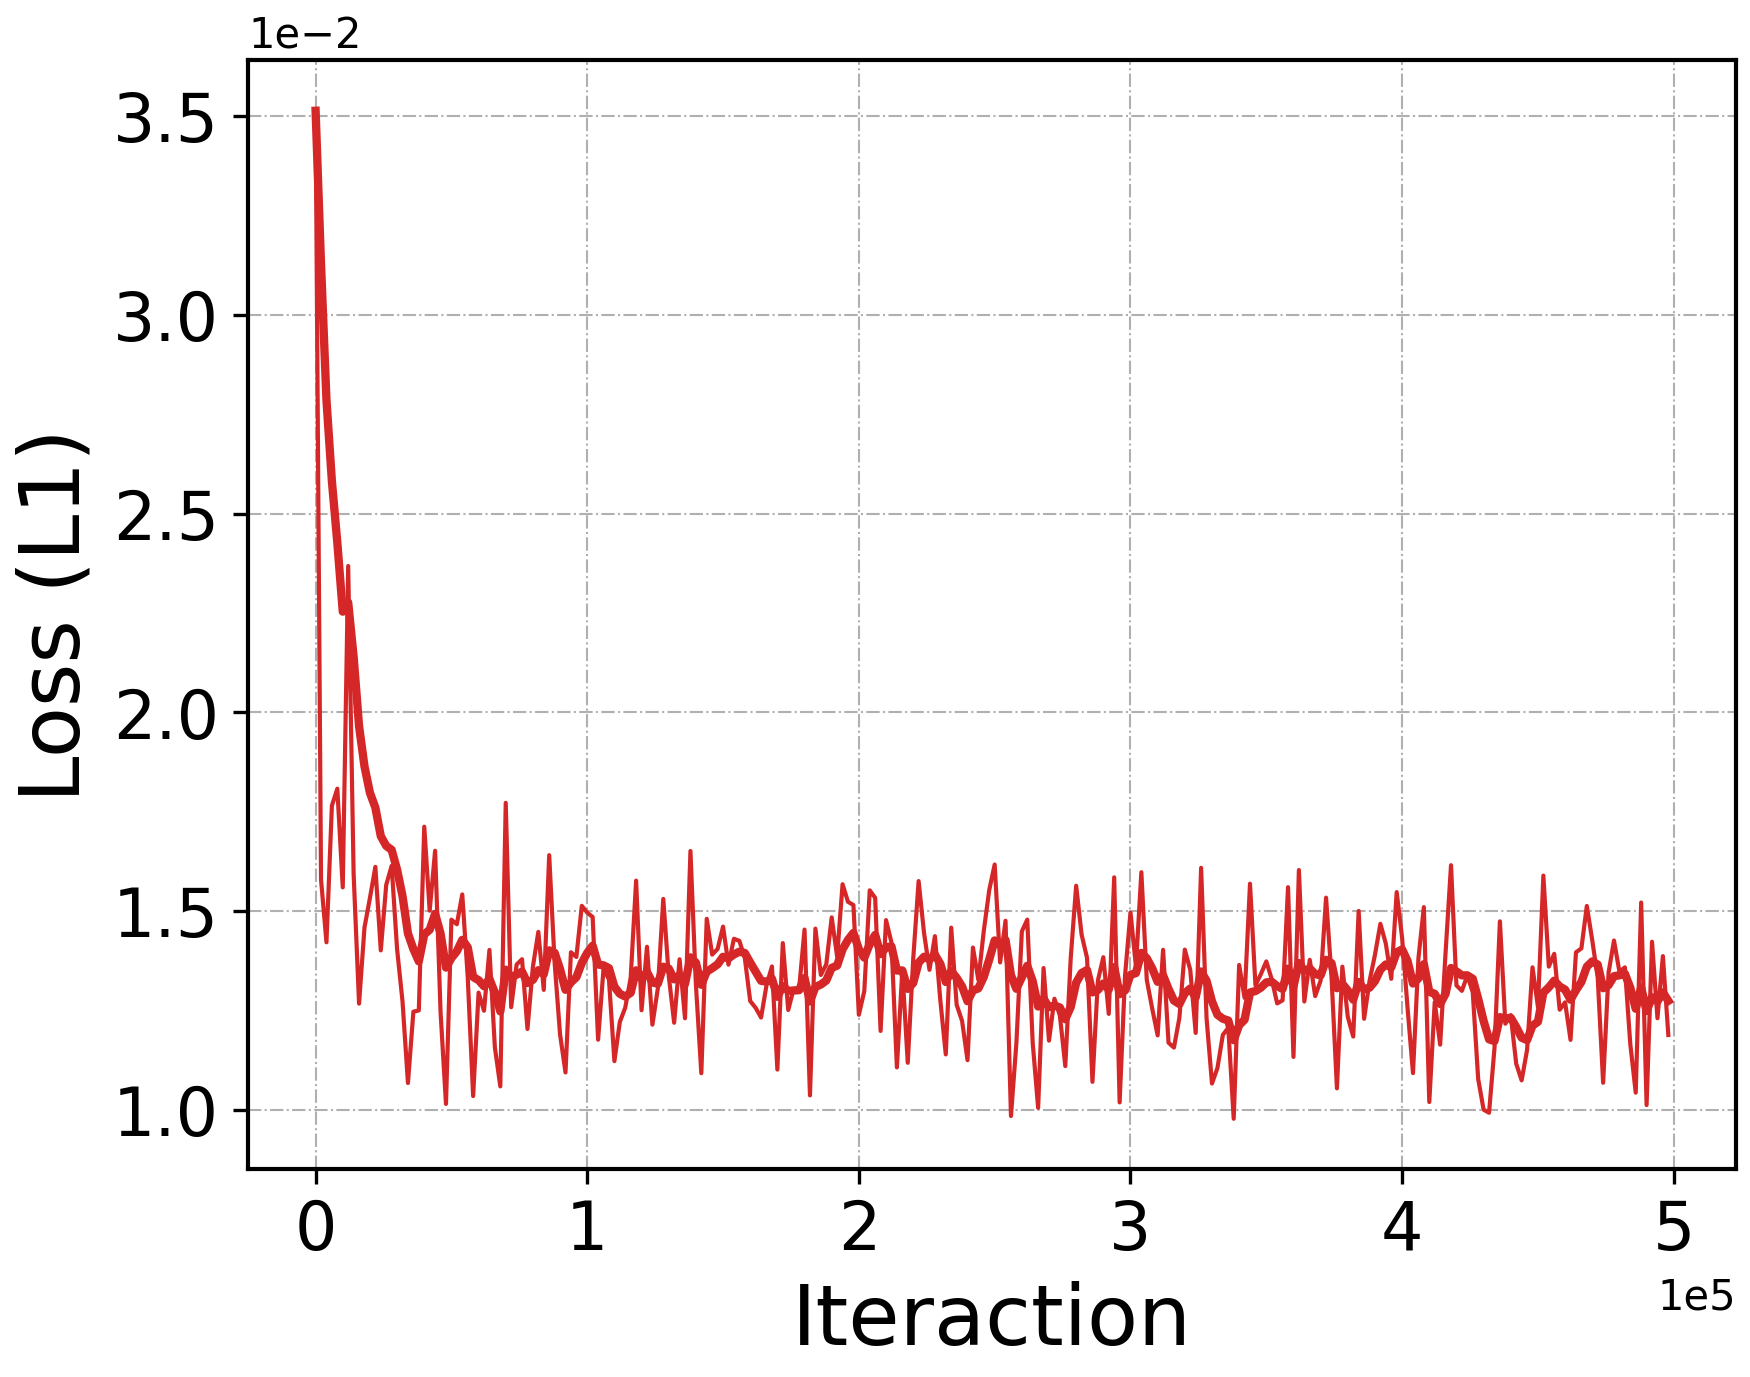} & \includegraphics[width=0.5\linewidth]{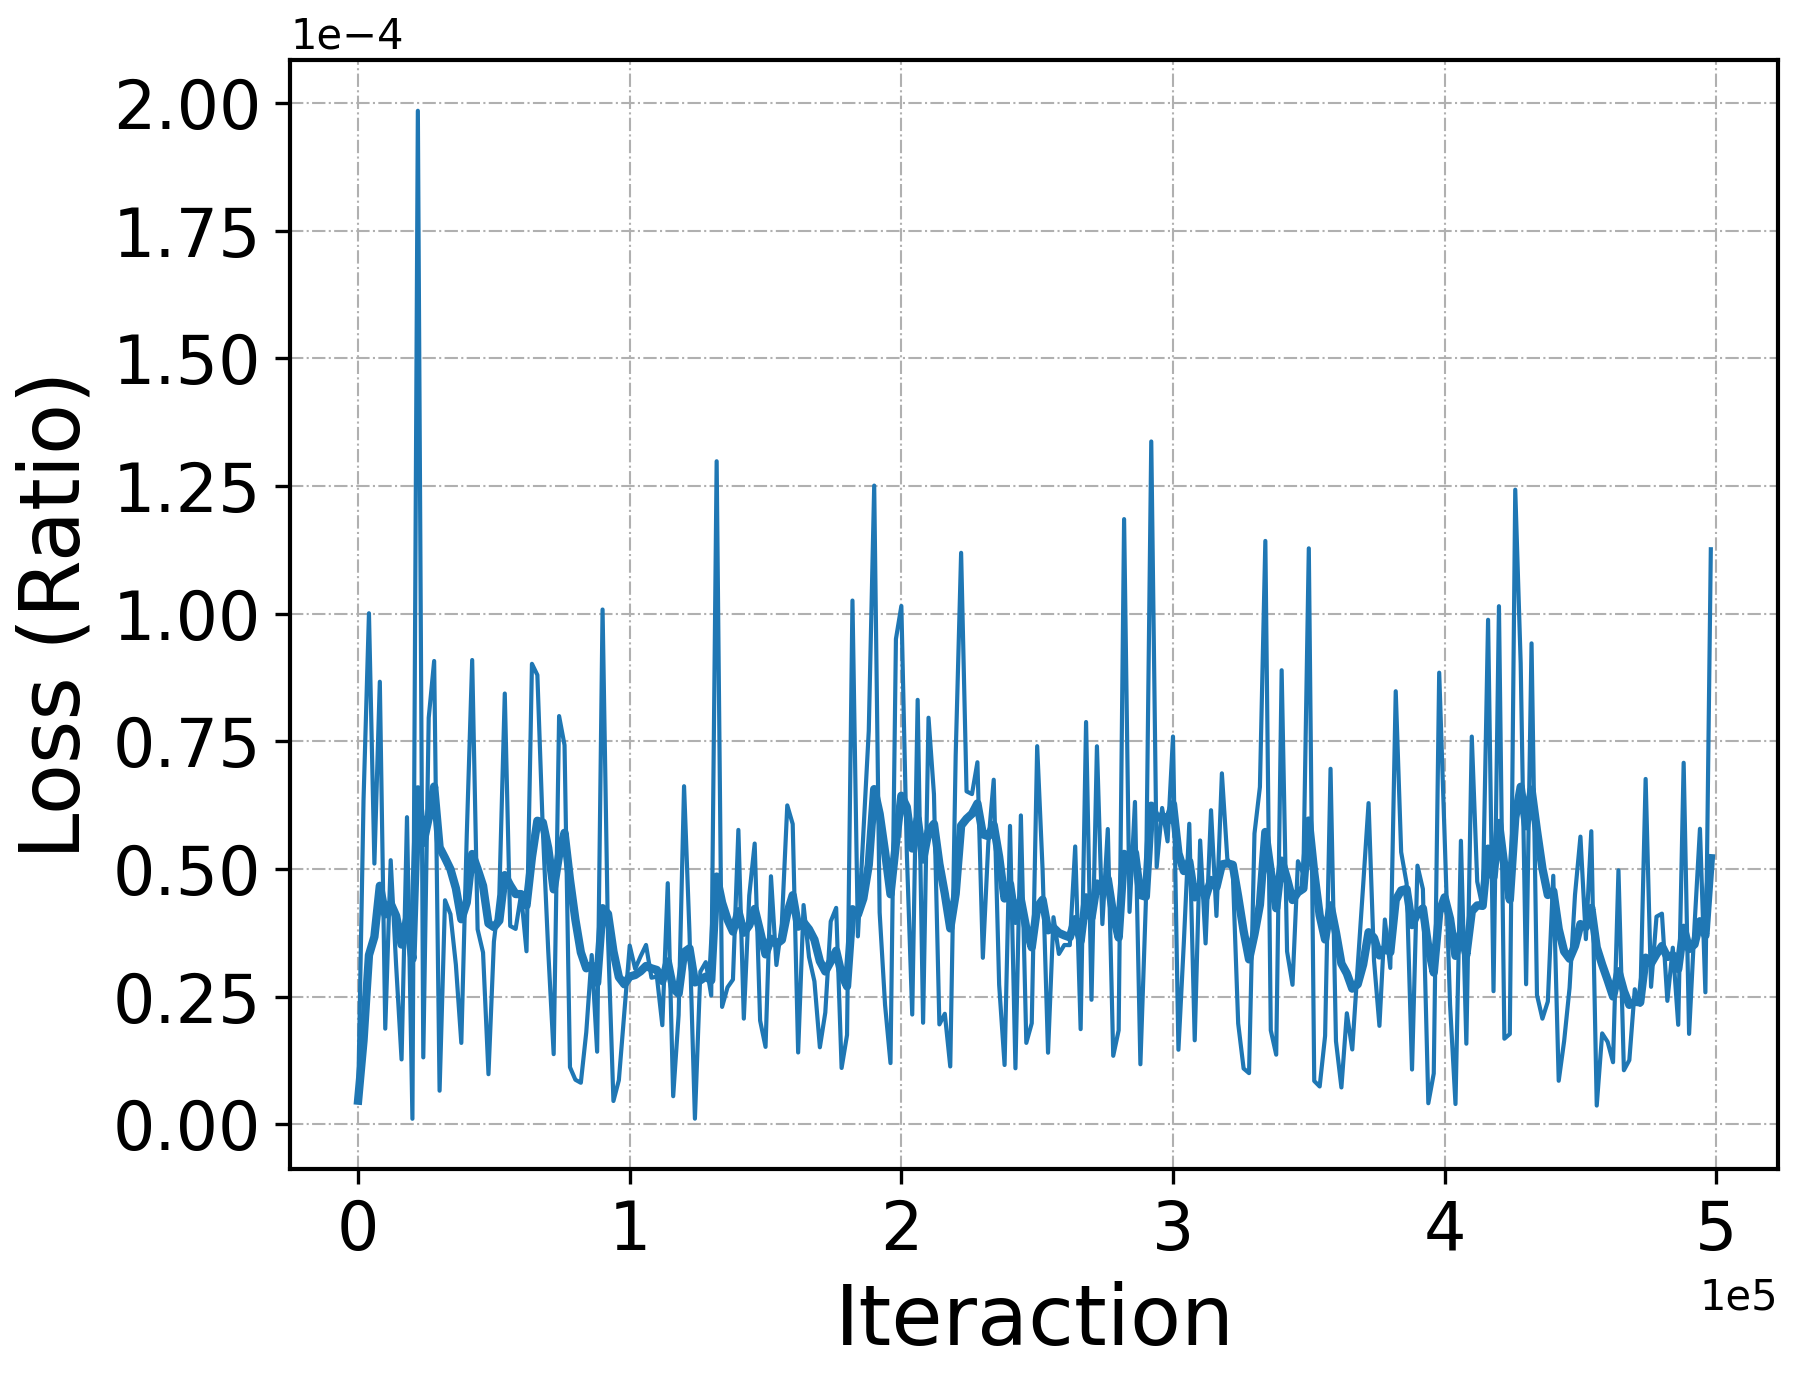} \\
             (a) $\ell_1$  & (b) $\ell_\etens{ratio}$\quad\quad\quad\quad\quad \\
             \includegraphics[width=0.48\linewidth]{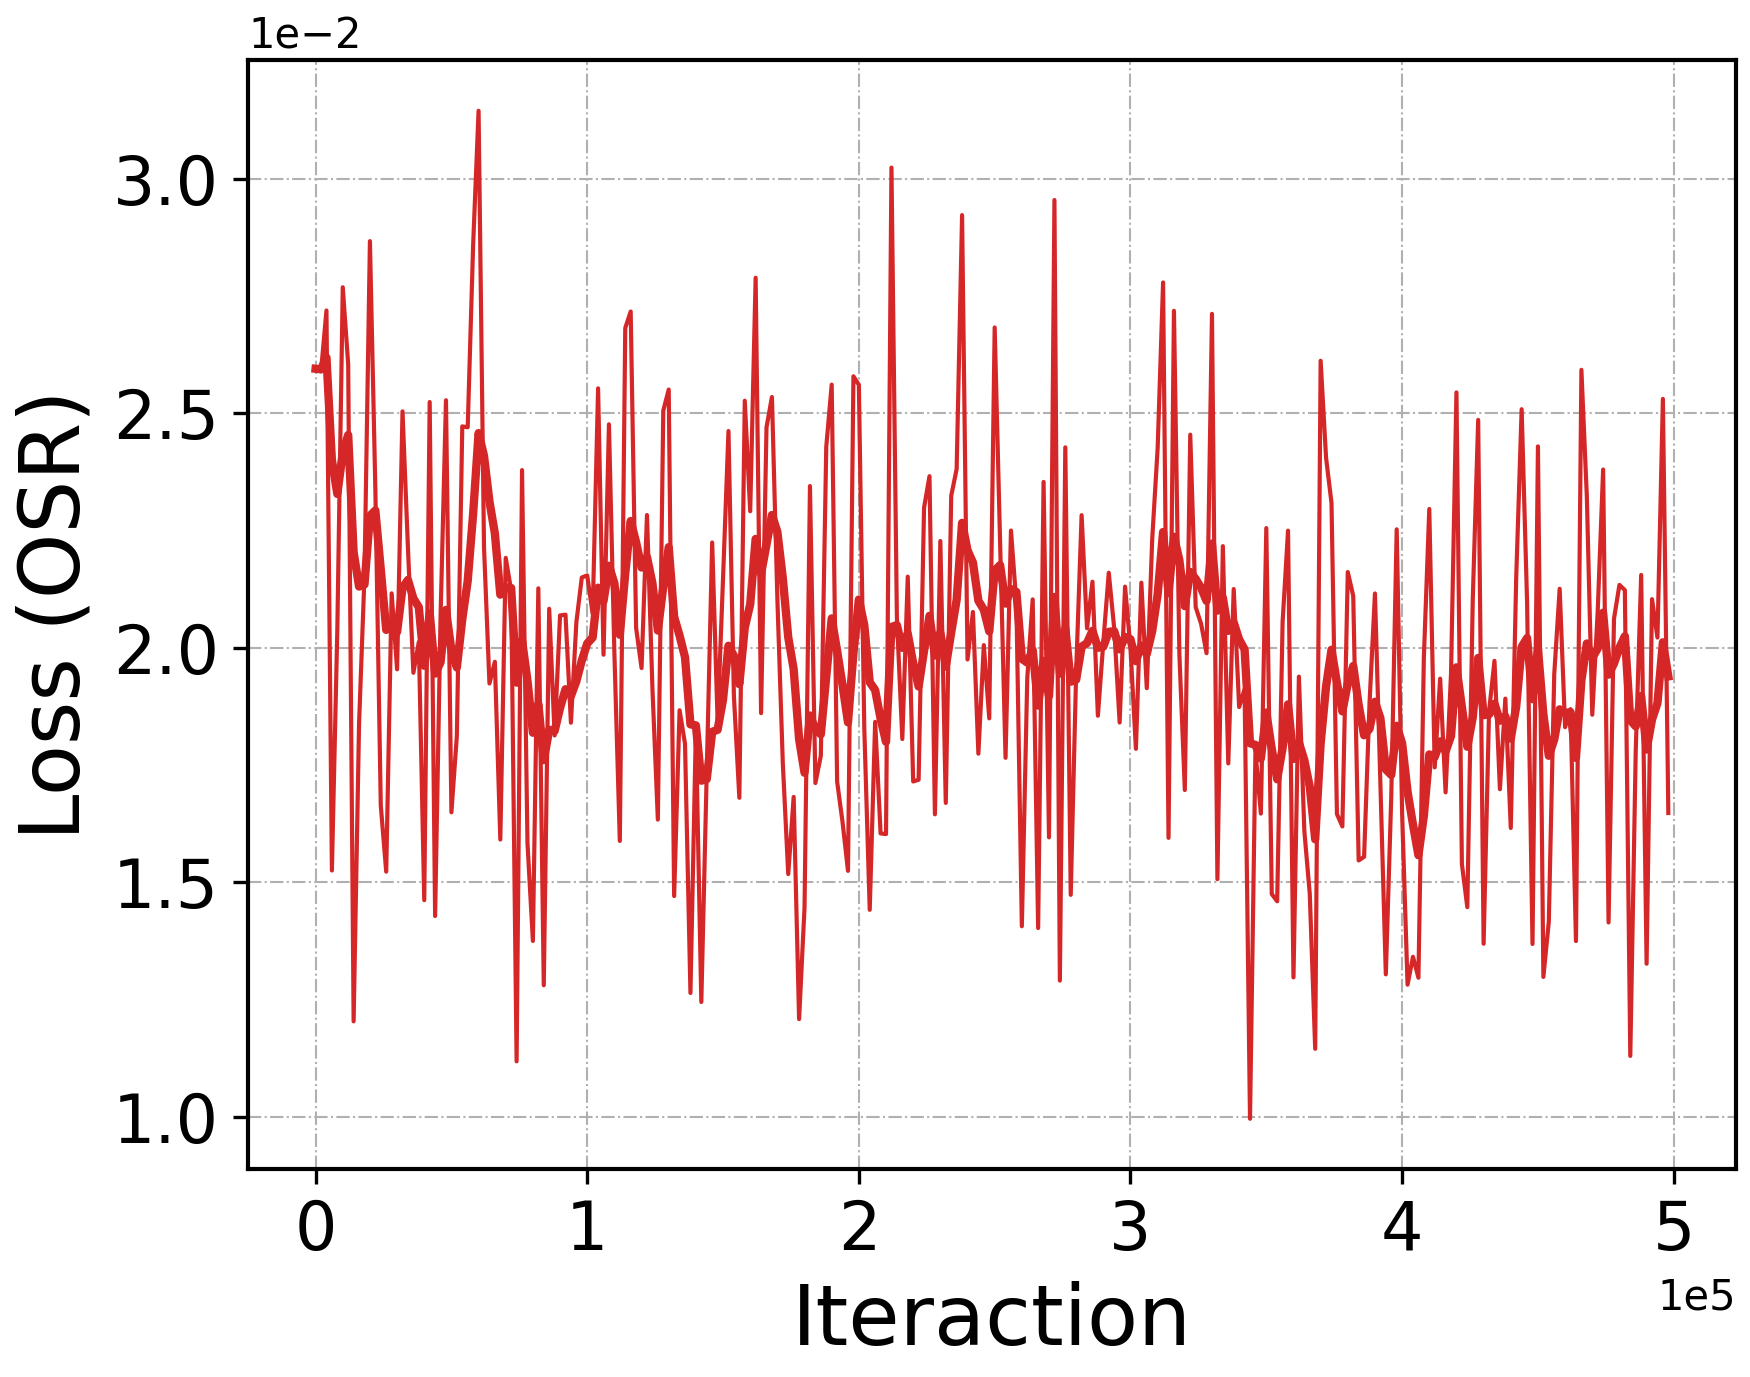} & \includegraphics[width=0.47\linewidth]{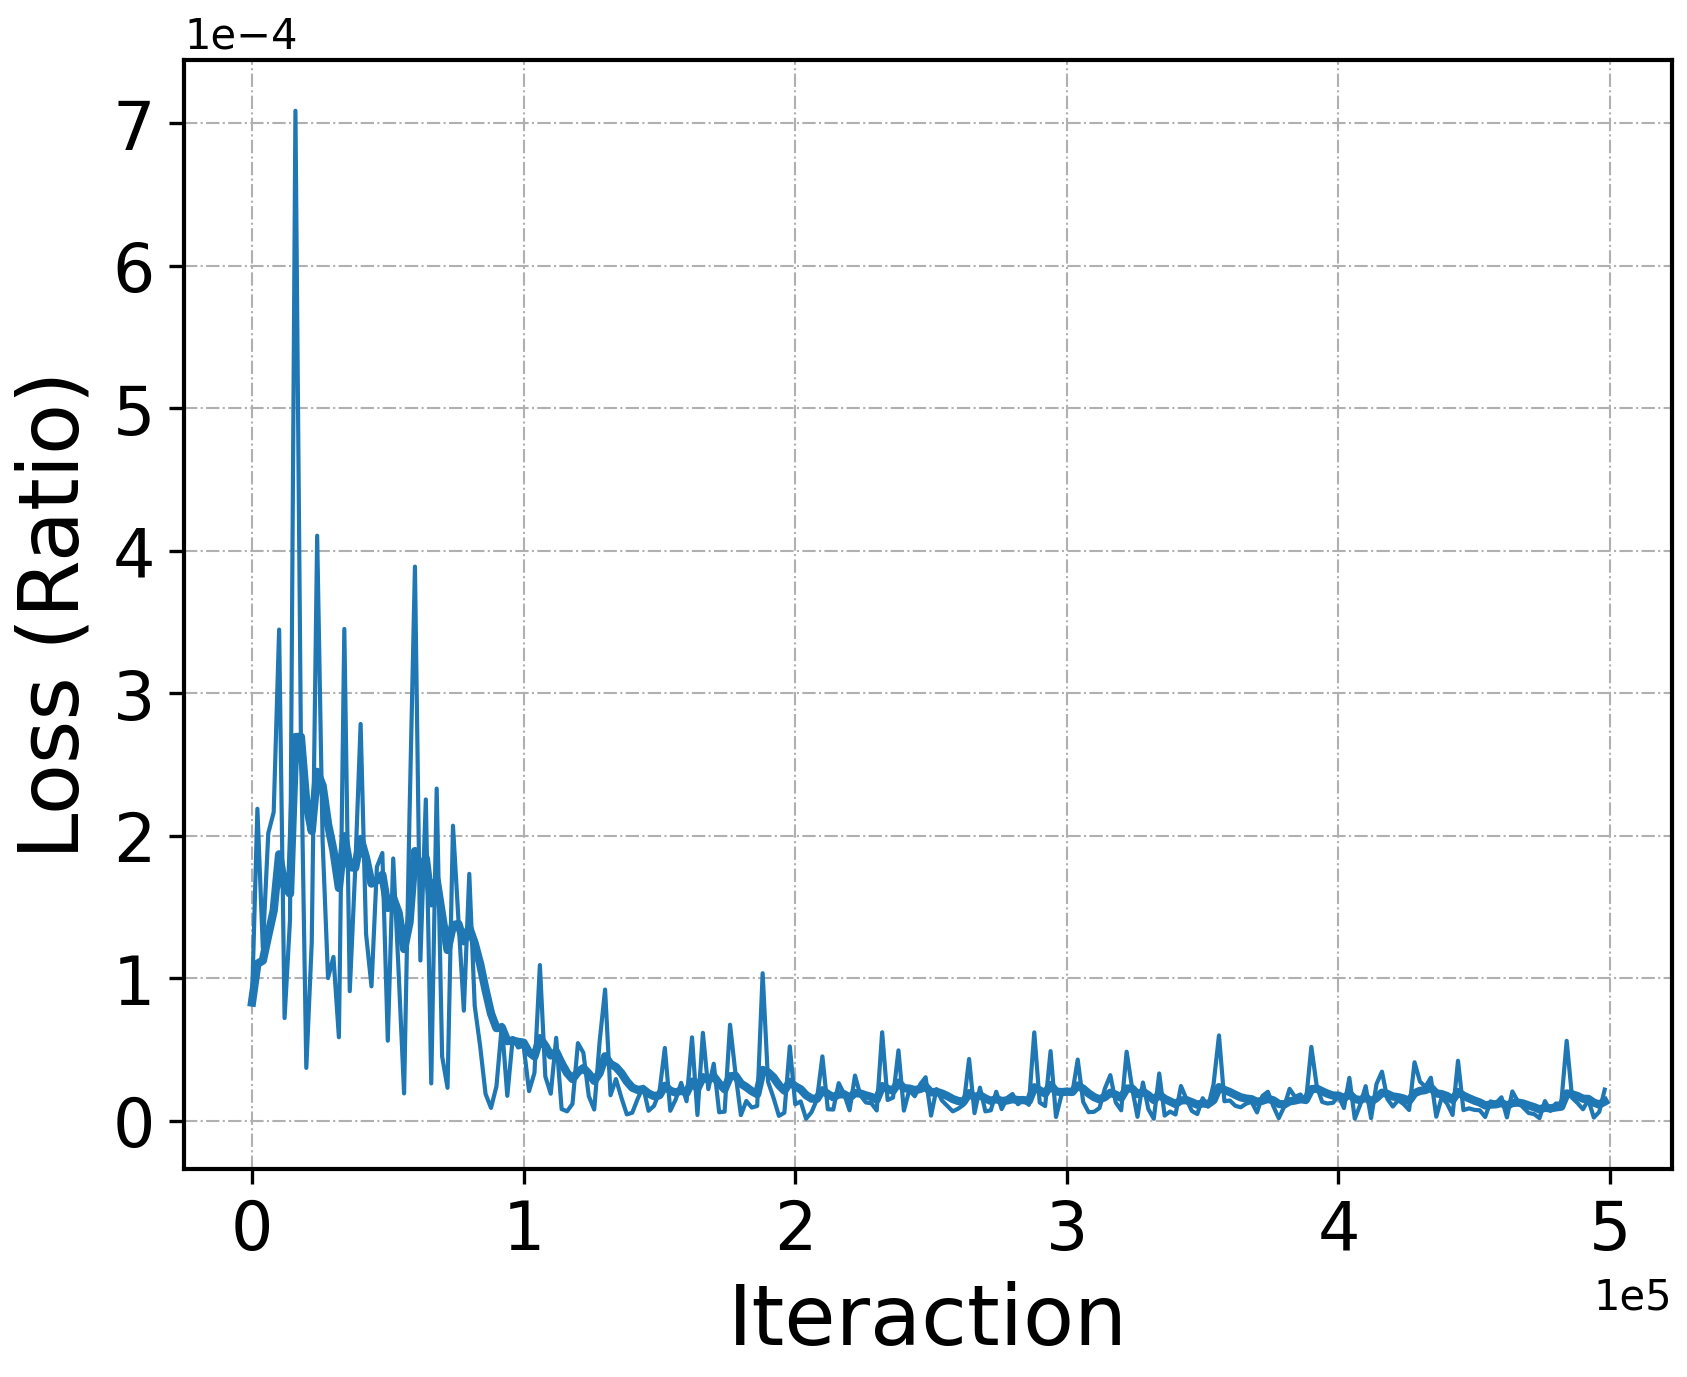} \\
             (c) $\ell_\etens{OSR}$  & (d) $\ell_\etens{ratio}$\quad\quad\quad\quad\quad
    \end{tabular}
    \caption{The loss curves for classic SR (a, b) and ODI SR (c, d).}
    \label{fig:loss}
\end{figure}

\subsection{Training Loss}
\noindent\textbf{Training Loss for ODI SR}. Based on LAU-Net~\cite{LAU-Net} and OSRT~\cite{OSRT}, we utilize the weighted $\ell_1$ loss for reconstruction. Given the input LR-HR pairs $\{I^\etens{LR}_i,I^\etens{HR}_i\}_{i=1}^N$, this calculation can be formulated by:
\begin{equation}
    \ell_\etens{OSR} = \frac{1}{N}\sum^N_{i=1}\left\| \rmW_j\left( \rmI^\etens{HR}_i - f_\etens{CAMixerSR}(\rmI^\etens{LR}_i) \right)\right\|_1,
\end{equation}
where the $\rmW_j$ is the  weight matrix
which defines the importance of each pixel according to its latitude. Given the latitude of the $p$-th row in $\rmW_j$ is $l$, following~\cite{LAU-Net}, we calculate its weight by $cos(\frac{l+0.5-H/2}{H}\pi)$. Similar to the classic SR task, we simply sum the $\ell_\etens{OSR}$ and $\ell_\etens{ratio}$ as the overall loss to train model for ODI SR.

\noindent\textbf{More Discussion}. We visualize the loss curves in~\cref{fig:loss} with two different tasks: classic SR and ODI SR task. Generally, for $\ell_\etens{ratio}$, the curve for ODI-SR is more reasonable and stable since 360$^{\circ}$ images have more plain area at high latitude while the density of complex area is random for images from classic SR datasets.
This property also induces the difference of $\ell_1$ and $\ell_\etens{OSR}$, where (a) is smoothly descended with fewer oscillations than (c).

\subsection{Texture Inconsistency}
The texture inconsistency may induce a huge performance drop since the CAMixer dynamically selects ``details'' tokens to calculate WSA. As discussed in the main paper, we resolve the texture inconsistency from two perspectives. 1) Design, we utilize the convolutional spatial/channel attention acting as a simple alignment for attentive features. 2) Training, the network itself learns to harmonize the feature by distributing CAMixer processing varied tokens. In \cref{fig:R2}, we offer heatmaps to show how these strategies work to erase the potential inconsistency. Specifically, for the model with convolutional attention, the difference between complex and simple tokens is alleviated to a large extent but still exists for uncoordinated patches. Then, as (b) illustrates, CAMixers of different layers hierarchically erase the inconsistency. 

\section{More Results}
\subsection{More Visualization of Predicted Mask}
In \cref{fig:1}, we present more visual results of the predicted mask with $\gamma$=0.5. For images with plenty of plain areas, our CAMixer can adopt eligible partitions for SA/Conv. However, two defects remain to be solved in our future work. 1) The fixed $\gamma$ is not flexible for images with excessively complex/simple textures. 2) The partition is learned from data without guidance, while some plain areas, \eg, human face, deserve more ``attention". In the future, we will continue to refine CAMixer with the adjustable ratio $\gamma$ and the human-guiding partition.

\begin{figure}
\fontsize{8.5pt}{0pt}\selectfont
\tabcolsep=0pt
    \centering
    \begin{tabular}{cccccc}
         \includegraphics[width=0.165\linewidth,height=0.113\linewidth]{Figure/mask4/temp3.png} 
         & \includegraphics[width=0.165\linewidth,height=0.113\linewidth]{Figure/mask4/temp6.png}
         & \includegraphics[width=0.165\linewidth,height=0.113\linewidth]{Figure/mask4/temp9.png}
         & \includegraphics[width=0.165\linewidth,height=0.113\linewidth]{Figure/mask4/temp13.png}
         & \includegraphics[width=0.165\linewidth,height=0.113\linewidth]{Figure/mask4/temp18.png}
         & \includegraphics[width=0.165\linewidth,height=0.113\linewidth]{Figure/mask4/temp19.png}\\
         \includegraphics[width=0.165\linewidth,height=0.113\linewidth]{Figure/mask5/temp3.png} 
         & \includegraphics[width=0.165\linewidth,height=0.113\linewidth]{Figure/mask5/temp6.png}
         & \includegraphics[width=0.165\linewidth,height=0.113\linewidth]{Figure/mask5/temp9.png}
         & \includegraphics[width=0.165\linewidth,height=0.113\linewidth]{Figure/mask5/temp13.png}
         & \includegraphics[width=0.165\linewidth,height=0.113\linewidth]{Figure/mask5/temp18.png}
         & \includegraphics[width=0.165\linewidth,height=0.113\linewidth]{Figure/mask5/temp19.png}\\
         \includegraphics[width=0.165\linewidth,height=0.113\linewidth]{Figure/mask6/temp3.png} 
         & \includegraphics[width=0.165\linewidth,height=0.113\linewidth]{Figure/mask6/temp6.png}
         & \includegraphics[width=0.165\linewidth,height=0.113\linewidth]{Figure/mask6/temp9.png}
         & \includegraphics[width=0.165\linewidth,height=0.113\linewidth]{Figure/mask6/temp13.png}
         & \includegraphics[width=0.165\linewidth,height=0.113\linewidth]{Figure/mask6/temp18.png}
         & \includegraphics[width=0.165\linewidth,height=0.113\linewidth]{Figure/mask6/temp19.png}\\
         \includegraphics[width=0.165\linewidth,height=0.113\linewidth]{Figure/mask7/temp3.png} 
         & \includegraphics[width=0.165\linewidth,height=0.113\linewidth]{Figure/mask7/temp6.png}
         & \includegraphics[width=0.165\linewidth,height=0.113\linewidth]{Figure/mask7/temp9.png}
         & \includegraphics[width=0.165\linewidth,height=0.113\linewidth]{Figure/mask7/temp13.png}
         & \includegraphics[width=0.165\linewidth,height=0.113\linewidth]{Figure/mask7/temp18.png}
         & \includegraphics[width=0.165\linewidth,height=0.113\linewidth]{Figure/mask7/temp19.png}\\
         \includegraphics[width=0.165\linewidth,height=0.113\linewidth]{Figure/mask8/temp3.png} 
         & \includegraphics[width=0.165\linewidth,height=0.113\linewidth]{Figure/mask8/temp6.png}
         & \includegraphics[width=0.165\linewidth,height=0.113\linewidth]{Figure/mask8/temp9.png}
         & \includegraphics[width=0.165\linewidth,height=0.113\linewidth]{Figure/mask8/temp13.png}
         & \includegraphics[width=0.165\linewidth,height=0.113\linewidth]{Figure/mask8/temp18.png}
         & \includegraphics[width=0.165\linewidth,height=0.113\linewidth]{Figure/mask8/temp19.png}\\
    \end{tabular}
    \caption{More visualizations of progressively classified tokens.}
    \label{fig:1}
\end{figure}

\begin{figure}[t]
\scriptsize
\centering
\tabcolsep=0.1pt
\begin{tabular}{cc}
\includegraphics[height=0.17\linewidth]{Figure2/R1/cool.pdf} \\
(a) w/o and w/ Conv Attn \\
\includegraphics[height=0.17\linewidth]{Figure2/R1/hot.pdf}\\
(b) heatmaps for sampled \{4,8,14,20\}-th CAMixers  \\
\end{tabular}
\caption{Effects of convolutional attention and block schedule.}
\label{fig:R2}
\end{figure}

\subsection{Runtime Performance}
Initially, we show the runtime percentage for components of CAMixer in~\cref{fig:2}. Obviously, the self-attention branch is the main barrier (67.8\%) that constrains efficiency. Thus, CAMixer integrates content-aware routing to reduce the latency for attention.
We validate the runtime performance of the proposed CAMixer on efficient SR tasks with the same setting as the NTIRE ESR Challenge\footnote{\url{https://github.com/ofsoundof/NTIRE2022_ESR}}~\cite{li2022ntire}. In~\cref{tab:1}, we examine our CAMixerSR with varied devices on Urban100~\cite{Urban100}. We can observe that the training mode is slightly faster than the inference ($\gamma=1.00$) due to the inference executing an extra selection operation to classify tokens. For latency, when testing on CPU or weak GPU (\eg, T4), the latency reduction is similar to MAdds, \ie, 30\% for $\gamma=0.5$ and 40\% for $\gamma=0.25$. Due to device limitations, the consumer-grade GPUs, \eg GTX and RTX series, are not included, which may attain larger improvements than T4. For more powerful GPU (\eg, V100), the runtime decrease is rather limited, less than 10\%. The results indicate that, on devices with low FLOPS barriers, our CAMixer can effectively save the computations and running time.

\begin{table}[t]
    \centering
    \fontsize{8.5pt}{9.5pt}\selectfont
    \tabcolsep=2pt
    \begin{tabular}{l|c|ccc}
    \whline
    \multirow{2}{*}{Device} & \multirow{2}{*}{Training} & \multicolumn{3}{c}{Inference}\\
    & & $\gamma=1.00$ & $\gamma=0.50$ & $\gamma=0.25$ \\
    \whline
    \#MAdds &- & 77.9G & 53.8G (69\%) & 43.0G (55\%)\\
    \whline
    CPU$^\dagger$ & 11.6s &  13.2s  & 9.6s (73\%) & 9.0s (68\%) \\
    Tesla T4  & 214.9ms  & 227.7ms & 180.6ms (79\%) & 177.3ms (78\%)\\
    Tesla A10 & 106.3ms & 113.4ms & 97.4ms (86\%) & 91.6ms (81\%)\\
    Tesla V100 & 95.3ms & 97.4ms & 90.2ms (92\%) & 88.7ms (91\%) \\
    % Tesla A100 & \\
    \whline
    \end{tabular}
    \caption{Runtime performance for CAMixerSR with various $\gamma$ on multiple devices. Mult-Adds (MAdds) are measured under the setting of upscaling the image to 1280$\times$720. The latency is the average runtime for single image SR on Urban100~\cite{Urban100}. ``$\dagger$'' uses Set5~\cite{Set5} and single core of Intel Xeon Platinum 8336C@2.3GHz.}
    \label{tab:1}
\end{table}

\begin{figure}
    \centering
    \includegraphics[width=0.7\linewidth]{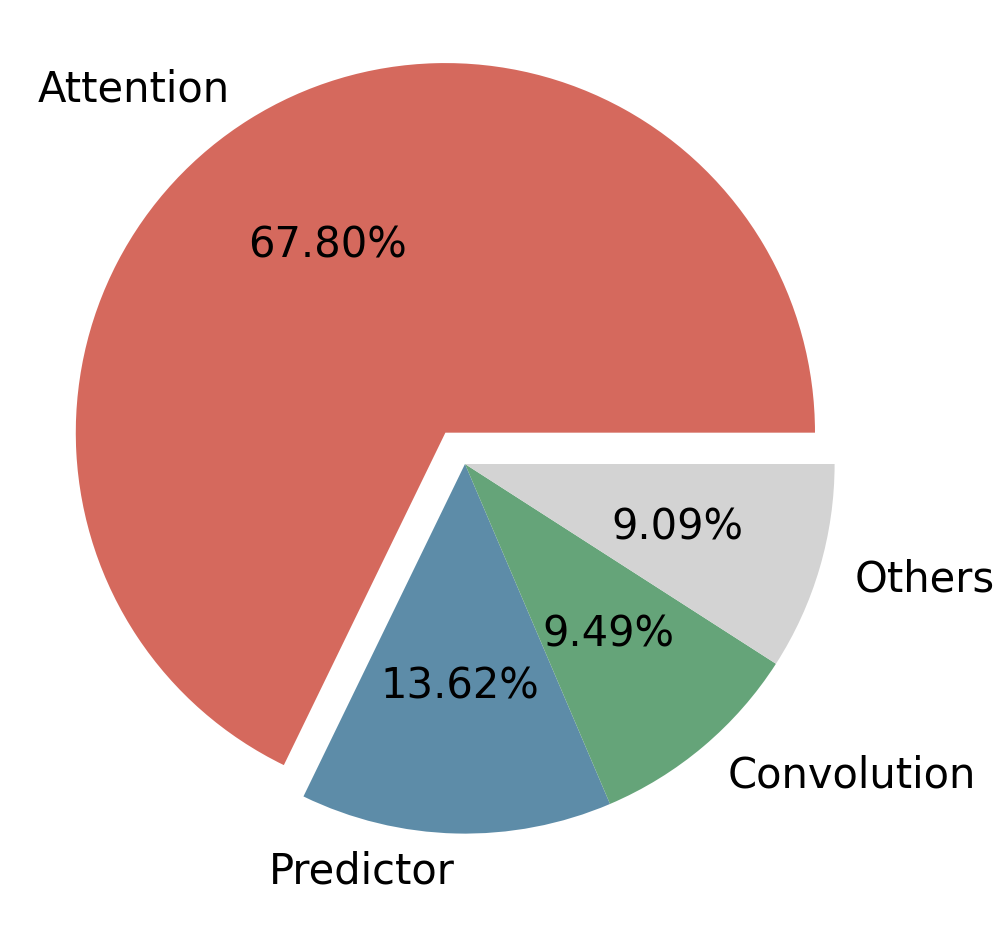}
    \caption{Runtime percentage of varied components (predictor, attention, convolution, and others) of CAMixer ($\gamma=1.0$).}
    \label{fig:2}
\end{figure}

\begin{figure}
    \centering
    \fontsize{8.5pt}{9.5pt}\selectfont
    \tabcolsep=1pt
    \begin{tabular}{cccccc}
\includegraphics[width=0.155\linewidth]{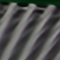}
& \includegraphics[width=0.155\linewidth]{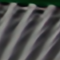} 
& \includegraphics[width=0.155\linewidth]{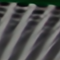}  
& \includegraphics[width=0.155\linewidth]{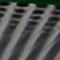} 
& \includegraphics[width=0.155\linewidth]{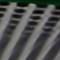} 
& \includegraphics[width=0.155\linewidth]{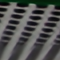} \\
$\gamma= 0.0$ & $\gamma=0.1$ & $\gamma=0.2$ & $\gamma=0.3$ & $\gamma=0.4$ & $\gamma=0.5$\\
\includegraphics[width=0.155\linewidth]{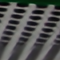} 
& \includegraphics[width=0.155\linewidth]{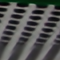} 
& \includegraphics[width=0.155\linewidth]{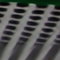} 
& \includegraphics[width=0.155\linewidth]{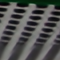} 
& \includegraphics[width=0.155\linewidth]{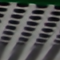} 
& \includegraphics[width=0.155\linewidth]{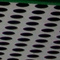} \\
$\gamma=0.6$ & $\gamma=0.7$ & $\gamma=0.8$ & $\gamma=0.9$ & $\gamma=1.0$ & HR\\
\end{tabular}
    \caption{Visual comparison for varied attention ratio $\gamma$.}
    \label{fig:3}
\end{figure}

\begin{table*}[!t]\scriptsize
\center
\begin{center}
\caption{Quantitative comparison (PSNR) for CAMixerSR-\textbf{Small}/\textbf{Medium}/\textbf{Base} with varied ratio $\gamma$ on F2K, Test2K, Test4K, and Test8K.}

\label{tab:3}
  % Here 1/2
\small
\footnotesize
\fontsize{8.5pt}{9.5pt}\selectfont
\tabcolsep=5.5pt
\begin{tabular}{ccc|cc|cc|cc|cc}
\whline
& {Ratio $\gamma$}  & {\#Params} & F2K & {\#FLOPs}  & Test2K & {\#FLOPs} & Test4K & {\#FLOPs}  & Test8K & {\#FLOPs}% & Manga% & Manga
\\
\whline
% & Original & 1.5M
% & 29.01
% & 5.20G\,(100\%)
% & 26.19
% & 5.20G\,(100\%)
% & 27.65
% & 5.20G\,(100\%)
% & 33.50
% & 5.20G\,(100\%)
% \\
% \rowcolor{tablered} 
% & ClassSR~\cite{ClassSR} & 3.1M
% & 29.02
% & 3.43G\,(66\%) 
% & 26.20
% & 3.62G\,(70\%)
% & 27.66
% & 3.30G\,(63\%)
% & 33.50
% & 2.70G\,(52\%)
% \\
% \rowcolor{tablegreen}
% & ARM-L~\cite{ARM}\quad\quad & 
% & 29.03
% & 4.23G\,(81\%)
% & 26.21
% & 4.00G\,(77\%)
% & 27.66
% & 3.41G\,(66\%)
% & 33.52
% & 3.24G\,(62\%)
% \\
% \rowcolor{tablegreen}
% & ARM-M~\cite{ARM}\quad\quad & 1.5M
% & 29.01
% & 3.59G\,(69\%)
% & 26.20
% & 3.48G\,(67\%)
% & 27.65
% & 3.24G\,(62\%)
% & 33.50
% & 2.47G\,(48\%)
% \\
% \rowcolor{tablegreen} 
% \multirow{-5}{*}{\rotatebox{90}{SRResNet}}
% & ARM-S~\cite{ARM}\quad\quad & 
% & 28.97
% & 2.74G\,(53\%)
% & 26.18
% & 2.87G\,(55\%)
% & 27.63
% & 2.77G\,(53\%)
% & 33.46
% & 1.83G\,(35\%)
% \\
% \hline
% & IMDN~\cite{IMDN} 
% & 715K 
% & 29.03
% & 729M
% & 26.19
% & 729M
% & 27.65
% & 729M
% & 33.57
% & 729M
% \\
% & SwinIR-light~\cite{SwinIR} 
% & 930K 
% & 29.24
% & 1.05G
% & 26.33
% & 1.05G
% & 27.79
% & 1.05G
% & 33.67
% & 1.05G
% \\
% \hline
% \rowcolor{tableblue} 
& 1.00 &  
& 29.12
& 894M\,(100\%)
& 26.26
& 894M\,(100\%)
& 27.73
& 894M\,(100\%)
& 33.66
& 894M\,(100\%)
% & \textbf{39.70}
\\
% \rowcolor{tableblue} 
& 0.50  &  
& 29.08
& 652M\,(73\%)
& 26.24
& 652M\,(73\%)
& 27.70
& 652M\,(73\%)
& 33.63
& 652M\,(73\%)
% & \textbf{39.70}
\\
% \rowcolor{tableblue} 
& 0.25  &  
& 28.98
& 532M\,(59\%)
& 26.18
& 532M\,(59\%)
& 27.63
& 532M\,(59\%)
& 33.55
& 532M\,(59\%)
% & \textbf{39.70}
\\
% \rowcolor{tableblue} 
\multirow{-4}{*}{\rotatebox{90}{\textbf{Small}}}
& 0.00  & \multirow{-4}{*}{351K} 
& 28.83
& 410M\,(46\%)
& 26.10
& 410M\,(46\%)
& 27.52
& 410M\,(46\%)
& 33.43
& 410M\,(46\%)
% & \textbf{39.70}
\\
\hline
% \rowcolor{tableblue} 
& 1.00 &  
& 29.20
& 1.37G\,(100\%)
& 26.32
& 1.37G\,(100\%)
& 27.80
& 1.37G\,(100\%)
& 33.72
& 1.37G\,(100\%)
% & \textbf{39.70}
\\
% \rowcolor{tableblue} 
& 0.50  &  
& 29.18
& 1.03G\,(75\%)
& 26.30
& 1.03G\,(75\%)
& 27.79
& 1.03G\,(75\%)
& 33.71
& 1.03G\,(75\%)
% & \textbf{39.70}
\\
% \rowcolor{tableblue} 
& 0.25 &  
& 29.11
& 858M\,(62\%)
& 26.26
& 858M\,(62\%)
& 27.74
& 858M\,(62\%)
& 33.66
& 858M\,(62\%)
% & \textbf{39.70}
\\
% \rowcolor{tableblue} 
\multirow{-4}{*}{\rotatebox{90}{\textbf{Medium}}}
& 0.00 & \multirow{-4}{*}{535K} 
& 28.92
& 686M\,(50\%)
& 26.15
& 686M\,(50\%)
& 27.59
& 686M\,(50\%)
& 33.50
& 686M\,(50\%)
% & \textbf{39.70}
\\
\hline
% \rowcolor{tableblue} 
&    1.00 &  
& 29.35
& 1.96G\,(100\%)
& 26.40
& 1.96G\,(100\%)
& 27.89
& 1.96G\,(100\%)
&33.81
& 1.96G\,(100\%)
% & \textbf{39.70}
\\
% \rowcolor{tableblue} 
& 0.50 &  
& 29.32
& 1.49G\,(76\%)
& 26.39
& 1.49G\,(76\%)
& 27.87
& 1.49G\,(76\%)
& 33.81
& 1.49G\,(76\%)
% & \textbf{39.70}
\\
% \rowcolor{tableblue} 
& 0.25 &  
& 29.26
& 1.26G\,(65\%)
& 26.35
& 1.26G\,(65\%)
& 27.83
& 1.26G\,(65\%)
& 33.77
& 1.26G\,(65\%)
% & \textbf{39.70}
\\
% \rowcolor{tableblue} 
\multirow{-4}{*}{\rotatebox{90}{\textbf{Base}}}
& 0.00 & \multirow{-4}{*}{765K}
& 29.08
& 1.03G\,(53\%)
& 26.23
& 1.03G\,(53\%)
& 27.70
& 1.03G\,(53\%)
& 33.63
& 1.03G\,(53\%)
% & \textbf{39.70}
\\
% % \rowcolor{tableblue} 
% \multirow{-5}{*}{\rotatebox{90}{\textbf{CASR}}}
% &   ClassSR &  \multirow{-5}{*}{765K}
% & 29.18
% & 718M\,(73\%)
% & 26.28
% & 758M\,(77\%)
% & 27.70
% & 1.03G\,(53\%)
% & 33.63
% & 1.03G\,(53\%)
% % & \textbf{39.70}
% \\
% \hline
% & RCAN~\cite{RCAN} & 15.6M
% & -
% & -
% & 26.39
% & 32.60G\,(100\%)
% & 27.89
% & 32.60G\,(100\%)
% & 33.76
% & 32.60G\,(100\%)
% % & \textbf{39.70}
% \\
% \rowcolor{tablered} 
% & ClassSR~\cite{ClassSR} & 30.1M
% & -
% & -
% & 26.39
% & 21.22G\,(65\%)
% & 27.88
% & 19.49G\,(60\%)
% & 33.73
% & 16.36G\,(50\%)
% \\
\whline
\end{tabular}
\end{center}
\end{table*}

\begin{table*}[!t]
\center
\small
\footnotesize
%\scriptsize
\fontsize{8.5pt}{9.5pt}\selectfont
\tabcolsep=5pt
\begin{center}
\caption{Quantitative comparison (average PSNR/SSIM, Parameters, and Mult-Adds) with varied ratio $\gamma$ for efficient image SR. Mult-Adds (MAdds) are measured under the setting of upscaling the image to 1280$\times$720. ``$\dagger$'' indicates using the DF2K~\cite{EDSR} training set.} 
% ``$\dagger$'' indicates using the DF2K~\cite{EDSR} augment training set.
\label{tab:4}
  % Here 1/2

\begin{tabular}{c|c|cc|c|c|c|c|c|c|c|c|c|c}
\whline
\multirow{2}{*}{Ratio $\gamma$} & \multirow{2}{*}{Scale} & \multirow{2}{*}{\#Params} & \multirow{2}{*}{\#MAdds}&  \multicolumn{2}{c|}{Set5~\cite{Set5}} &  \multicolumn{2}{c|}{Set14~\cite{Set14}} &  \multicolumn{2}{c|}{BSD100~\cite{B100}} &  \multicolumn{2}{c|}{Urban100~\cite{Urban100}} &  \multicolumn{2}{c}{Manga109~\cite{manga109}}
\\
\cline{5-14}
& &   &  & PSNR & SSIM & PSNR & SSIM & PSNR & SSIM & PSNR & SSIM  & PSNR & SSIM 
\\
%\hline
\whline
1.00   & $\times$2  
& & {294.1G} 
% & {306.6ms}
&  {{38.24}}
&  {\blue{0.9614}}
&  {{34.00}}
&  {\blue{0.9217}}
&  {{32.34}}
&  {{0.9017}}
&  {{32.97}}
&  {{0.9352}}
& {39.34}
& {0.9782}
\\
% \rowcolor{tableblue} 
0.50   & $\times$2  
& {746K} & {205.2G} 
% & {264.2ms}
&  {{38.23}}
&  {{0.9613}}
&  {{34.00}}
&  {{0.9214}}
&  {{32.34}}
&  {{0.9016}}
&  {{32.95}}
&  {{0.9348}}
& {39.32}
& {0.9781}
\\
% \rowcolor{tableblue} 
0.25  & $\times$2  
&  & {160.7G} 
% & {245.5ms}
&  {{38.16}}
&  {{0.9610}}
&  {{33.90}}
&  {{0.9206}}
&  {{32.31}}
&  {{0.9010}}
&  {{32.78}}
&  {{0.9329}}
& 39.25
& 0.9779
\\
\hline
% \rowcolor{lightgray} 
1.00$^\dagger$    & $\times$2  
& & {294.1G} 
% & {306.6ms}
&  {\red{38.28}}
&  {\red{0.9614}}
&  {\red{34.04}}
&  {\red{0.9218}}
&  {\red{32.37}}
&  {\red{0.9021}}
&  {\red{33.04}}
&  {\red{0.9364}}
& \red{39.50}
& \red{0.9788}
\\
% \rowcolor{lightgray} 
0.50$^\dagger$ & $\times$2  
& 746K  & {205.2G} 
% & {264.2ms}
&  {\blue{38.27}}
&  {\blue{0.9614}}
&  {\blue{34.03}}
&  {{0.9215}}
&  {\blue{32.36}}
&  {\blue{0.9019}}
&  {\blue{33.01}}
&  {\blue{0.9357}}
& \blue{39.49}
& \blue{0.9787}
\\
% \rowcolor{lightgray} 
0.25$^\dagger$  & $\times$2  
&  & {160.7G} 
% & {245.5ms}
&  {{38.21}}
&  {{0.9611}}
&  {{33.96}}
&  {{0.9208}}
&  {{32.33}}
&  {{0.9013}}
&  {{32.83}}
&  {{0.9336}}
& 39.43
& 0.9785
\\
\whline
1.00 & $\times$4  & & {77.9G} %
% & {97.4ms}
& {{32.51}}
& {{0.8992}}
& {{28.82}}
& {{0.7873}}
& {{27.73}}
& {{0.7421}}
& {{26.65}}
& {{0.8024}}
& {{31.20}}
& {\blue{0.9170}}
\\
% \rowcolor{tableblue} 
0.50 & $\times$4  & {765K} & {53.8G} %
% & {90.2ms}
& {{32.51}}
& {{0.8988}}
& {{28.82}}
& {{0.7870}}
& {{27.72}}
& {{0.7416}}
& {{26.63}}
& {{0.8012}}
& {{31.18}}
& {{0.9166}}
\\
% % \rowcolor{tableblue} 
0.25  & $\times$4  & & {43.0G} %
% & {88.7ms}
& {{32.45}}
& {{0.8978}}
& {{28.78}}
& {{0.7856}}
& {{27.69}}
& {{0.7401}}
& {{26.51}}
& {{0.7966}}
& {{31.06}}
& {{0.9148}}
\\
\hline
% \rowcolor{lightgray} 
1.00$^\dagger$ & $\times$4  &   & {77.9G} %
% & {97.4ms}
& {\red{32.60}}
& {\red{0.9003}}
& {\red{28.91}}
& {\red{0.7889}}
& {\red{27.78}}
& {\red{0.7434}}
& {\red{26.80}}
& {\red{0.8068}}
& {\red{31.42}}
& {{0.9168}}
\\
% \rowcolor{tableblue} 
0.50$^\dagger$ & $\times$4  & {765K} & {53.8G} %
% & {90.2ms}
& {\blue{32.58}}
& {\blue{0.9000}}
& {\blue{28.90}}
& {\blue{0.7885}}
& {\blue{27.77}}
& {\blue{0.7430}}
& {\blue{26.77}}
& {\blue{0.8055}}
& {\blue{31.41}}
& {\red{0.9171}}
\\
% \rowcolor{lightgray} 
0.25$^\dagger$  & $\times$4  &  & {43.0G} %
% & {88.7ms}
& {{32.47}}
& {{0.8986}}
& {{28.84}}
& {{0.7870}}
& {{27.73}}
& {{0.7413}}
& {{26.63}}
& {{0.8005}}
& {{31.31}}
& {{0.9168}}
\\
% EDSR~\cite{EDSR} & $\times$4  & 43680K & {2699.4G}
% &  -
% & 32.46
% & 0.8968 
% & 28.80 
% & 0.7876 
% & 27.71
% & 0.7420 
% & 26.64
% & 0.8033 
% & 31.02 
% & 0.9148
% \\
% Ada-EDSR~\cite{Ada} & $\times$4  & - & {2265.8G}
% &  -
% & 32.49
% & 0.8977 
% & 28.82 
% & 0.7880 
% & 27.71
% & 0.7410 
% & 26.58
% & 0.8011 
% & -
% & -
% \\
% FAD-EDSR~\cite{FAD} & $\times$4  & - & {1729.9G}
% &  -
% & 32.50
% & 0.8977 
% & 28.82 
% & 0.7880 
% & 27.73
% & 0.7438 
% & 26.70
% & 0.8049 
% & -
% & -
% \\
\whline 
\end{tabular}
\end{center}
\end{table*}

\begin{figure*}[!t]
    \centering
    \scriptsize
    \tabcolsep=2pt
    \begin{tabular}{cccccc}
         \multirow{-7}{*}{\includegraphics[width=0.36\linewidth,height=0.24\linewidth]{Figure/U078/Z.png}}
         & \includegraphics[width=0.11\linewidth,height=0.11\linewidth]{Figure/U078/0_HR.png} 
         & \includegraphics[width=0.11\linewidth,height=0.11\linewidth]{Figure/U078/1_IMDN.png} 
         & \includegraphics[width=0.11\linewidth,height=0.11\linewidth]{Figure/U078/2_FDIWN.png}
         & \includegraphics[width=0.11\linewidth,height=0.11\linewidth]{Figure/U078/10_CAMixer-O.png} 
         & \includegraphics[width=0.11\linewidth,height=0.11\linewidth]{Figure/U078/12_CAMixer-O.png} 
         \\
         & HR & IMDN~\cite{IMDN} & FDIWN~\cite{FDIWN} & \textbf{\algname{}}-\emph{O} & \textbf{\algname{}}$^\dagger$-\emph{O} \\
         % & &  16.69/5.20G & 17.26/32.60G & 17.26/729M & 18.99/1.96G \\
         & \includegraphics[width=0.11\linewidth,height=0.11\linewidth]{Figure/U078/4_ESRT.png} 
         & \includegraphics[width=0.11\linewidth,height=0.11\linewidth]{Figure/U078/5_SwinIR.png} 
         & \includegraphics[width=0.11\linewidth,height=0.11\linewidth]{Figure/U078/6_NGSwin.png}
         & \includegraphics[width=0.11\linewidth,height=0.11\linewidth]{Figure/U078/9_CAMixer.png} 
         & \includegraphics[width=0.11\linewidth,height=0.11\linewidth]{Figure/U078/11_CAMixer.png} 
         \\
          {\emph{078} from Urban100} & ESRT~\cite{ESRT} & SwinIR~\cite{SwinIR} & NGswin~\cite{NGSwin} & \textbf{\algname{}} & \textbf{\algname{}}$^\dagger$\\
         % \multirow{-7}{*}{\includegraphics[width=0.36\linewidth,height=0.24\linewidth]{Figure/U092/Z.png}}
         % & \includegraphics[width=0.11\linewidth,height=0.11\linewidth]{Figure/U092/0_HR.png} 
         % & \includegraphics[width=0.11\linewidth,height=0.11\linewidth]{Figure/U092/img_092_HR_x4_IMDN_x4.png} 
         % & \includegraphics[width=0.11\linewidth,height=0.11\linewidth]{Figure/U092/img_092_HR_x4_BSRN_x4.png}
         % & \includegraphics[width=0.11\linewidth,height=0.11\linewidth]{Figure/U092/img_092_HR_x4_OSR_x4_100_new.png} 
         % & \includegraphics[width=0.11\linewidth,height=0.11\linewidth]{Figure/U092/img_092_HR_x4_OSR_x4_100_DF2K.png} 
         % \\
         % & HR & IMDN~\cite{IMDN} & BSRN~\cite{BSRN} & \textbf{\algname{}}-\emph{O} & \textbf{\algname{}}$^\dagger$-\emph{O} \\
         % % & &  16.69/5.20G & 17.26/32.60G & 17.26/729M & 18.99/1.96G \\
         % & \includegraphics[width=0.11\linewidth,height=0.11\linewidth]{Figure/U092/ESRT.png} 
         % & \includegraphics[width=0.11\linewidth,height=0.11\linewidth]{Figure/U092/SwinIR.png} 
         % & \includegraphics[width=0.11\linewidth,height=0.11\linewidth]{Figure/U092/img_092_HR_x4_NGSwin_x4.png}
         % & \includegraphics[width=0.11\linewidth,height=0.11\linewidth]{Figure/U092/img_092_HR_x4_OSR_x4_050_new.png} 
         % & \includegraphics[width=0.11\linewidth,height=0.11\linewidth]{Figure/U092/img_092_HR_x4_OSR_x4_050_DF2K.png} 
         % \\
         %  {\emph{092} from Urban100} & ESRT~\cite{ESRT} & SwinIR~\cite{SwinIR} & NGswin~\cite{NGSwin} & \textbf{\algname{}} & \textbf{\algname{}}$^\dagger$\\
         % & &  15.88/3.43G & 16.56/21.22G & 16.69/1.05G & 18.83/1.49G 
         % \\
    \end{tabular}
    \caption{Visual comparison of \algname{} with other methods for $\times$4 task on Urban100 dataset.}
    \label{fig:ESR2}
\end{figure*}

\subsection{Large-Image SR}
\label{sec:1}
In~\cref{tab:3}, we offer more quantitative results of CAMixerSR with varied $\gamma$ on the Large-Image SR task. In the main paper, we manually set $\gamma=0.5$ to attain the promising trade-offs for three tasks. However, for the 8K task, further decreasing the ratio to 0.25 can save an additional 115M (10\%) calculations while inducing only 0.04dB drops. We also examine the models without using self-attention ($\gamma=0$). In detail, the non-attention models suffer about 0.3dB PSNR drops. In~\cref{fig:Test4K2}, we offer more visual comparisons between our CAMixerSR with other methods, where CAMixerSR obtains better restoration quality.
These results indicate that only details need more ``attention", and we only need to pay ``attention" to 25\%-50\% areas.

\begin{figure*}
    \centering
    \scriptsize
    \tabcolsep=2pt
    \begin{tabular}{cccccc}
         \multirow{-7}{*}{\includegraphics[width=0.36\linewidth,height=0.24\linewidth]{Figure/4K2/Z.png}}
         & \includegraphics[width=0.11\linewidth,height=0.11\linewidth]{Figure/4K2/0_HR.png} 
         & \includegraphics[width=0.11\linewidth,height=0.11\linewidth]{Figure/4K2/SRResNet.png} 
         & \includegraphics[width=0.11\linewidth,height=0.11\linewidth]{Figure/4K2/RCAN.png}
         & \includegraphics[width=0.11\linewidth,height=0.11\linewidth]{Figure/4K2/IMDN.png} 
         & \includegraphics[width=0.11\linewidth,height=0.11\linewidth]{Figure/4K2/CAMixer-O.png} 
         \\
         & HR & SRResNet-\emph{O}~\cite{SRGAN} & RCAN-\emph{O}~\cite{RCAN} & IMDN-\emph{O}~\cite{IMDN} & \textbf{\algname{}}-\emph{O} \\
         % & &  16.69/5.20G & 17.26/32.60G & 17.26/729M & 18.99/1.96G \\
         & \includegraphics[width=0.11\linewidth,height=0.11\linewidth]{Figure/4K2/LR.png} 
         & \includegraphics[width=0.11\linewidth,height=0.11\linewidth]{Figure/4K2/ClassSR-SRResNet.png} 
         & \includegraphics[width=0.11\linewidth,height=0.11\linewidth]{Figure/4K2/ClassSR-RCAN.png}
         & \includegraphics[width=0.11\linewidth,height=0.11\linewidth]{Figure/4K2/SwinIR.png} 
         & \includegraphics[width=0.11\linewidth,height=0.11\linewidth]{Figure/4K2/CAMixer.png} 
         \\
          {\emph{1303} from Test4K} &{LR} & SRResNet-\emph{ClassSR} & RCAN-\emph{ClassSR} & SwinIR-L-\emph{O}~\cite{SwinIR} & \textbf{\algname{}} \\
         % & &  15.88/3.43G & 16.56/21.22G & 16.69/1.05G & 18.83/1.49G 
         % \\
         \multirow{-7}{*}{\includegraphics[width=0.36\linewidth,height=0.24\linewidth]{Figure/4K3/Z.png}}
         & \includegraphics[width=0.11\linewidth,height=0.11\linewidth]{Figure/4K3/0_HR.png} 
         & \includegraphics[width=0.11\linewidth,height=0.11\linewidth]{Figure/4K3/SRResNet.png} 
         & \includegraphics[width=0.11\linewidth,height=0.11\linewidth]{Figure/4K3/RCAN.png}
         & \includegraphics[width=0.11\linewidth,height=0.11\linewidth]{Figure/4K3/IMDN.png} 
         & \includegraphics[width=0.11\linewidth,height=0.11\linewidth]{Figure/4K3/CAMixer-O.png} 
         \\
         & HR & SRResNet-\emph{O}~\cite{SRGAN} & RCAN-\emph{O}~\cite{RCAN} & IMDN-\emph{O}~\cite{IMDN} & \textbf{\algname{}}-\emph{O} \\
         % & &  16.69/5.20G & 17.26/32.60G & 17.26/729M & 18.99/1.96G \\
         & \includegraphics[width=0.11\linewidth,height=0.11\linewidth]{Figure/4K3/LR.png} 
         & \includegraphics[width=0.11\linewidth,height=0.11\linewidth]{Figure/4K3/ClassSR-SRResNet.png} 
         & \includegraphics[width=0.11\linewidth,height=0.11\linewidth]{Figure/4K3/ClassSR-RCAN.png}
         & \includegraphics[width=0.11\linewidth,height=0.11\linewidth]{Figure/4K3/SwinIR.png} 
         & \includegraphics[width=0.11\linewidth,height=0.11\linewidth]{Figure/4K3/CAMixer.png} 
         \\
          {\emph{1334} from Test4K} &{LR} & SRResNet-\emph{ClassSR} & RCAN-\emph{ClassSR} & SwinIR-L-\emph{O}~\cite{SwinIR} & \textbf{\algname{}} \\
        \multirow{-7}{*}{\includegraphics[width=0.36\linewidth,height=0.24\linewidth]{Figure/4K4/Z.png}}
         & \includegraphics[width=0.11\linewidth,height=0.11\linewidth]{Figure/4K4/0_HR.png} 
         & \includegraphics[width=0.11\linewidth,height=0.11\linewidth]{Figure/4K4/SRResNet.png} 
         & \includegraphics[width=0.11\linewidth,height=0.11\linewidth]{Figure/4K4/RCAN.png}
         & \includegraphics[width=0.11\linewidth,height=0.11\linewidth]{Figure/4K4/IMDN.png} 
         & \includegraphics[width=0.11\linewidth,height=0.11\linewidth]{Figure/4K4/CAMixer-O.png} 
         \\
         & HR & SRResNet-\emph{O}~\cite{SRGAN} & RCAN-\emph{O}~\cite{RCAN} & IMDN-\emph{O}~\cite{IMDN} & \textbf{\algname{}}-\emph{O} \\
         % & &  16.69/5.20G & 17.26/32.60G & 17.26/729M & 18.99/1.96G \\
         & \includegraphics[width=0.11\linewidth,height=0.11\linewidth]{Figure/4K4/LR.png} 
         & \includegraphics[width=0.11\linewidth,height=0.11\linewidth]{Figure/4K4/ClassSR-SRResNet.png} 
         & \includegraphics[width=0.11\linewidth,height=0.11\linewidth]{Figure/4K4/ClassSR-RCAN.png}
         & \includegraphics[width=0.11\linewidth,height=0.11\linewidth]{Figure/4K4/SwinIR.png} 
         & \includegraphics[width=0.11\linewidth,height=0.11\linewidth]{Figure/4K4/CAMixer.png} 
         \\
          {\emph{1341} from Test4K} &{LR} & SRResNet-\emph{ClassSR} & RCAN-\emph{ClassSR} & SwinIR-L-\emph{O}~\cite{SwinIR} & \textbf{\algname{}} \\
           \multirow{-7}{*}{\includegraphics[width=0.36\linewidth,height=0.24\linewidth]{Figure/2K/Z.png}}
         & \includegraphics[width=0.11\linewidth,height=0.11\linewidth]{Figure/2K/HR.png} 
         & \includegraphics[width=0.11\linewidth,height=0.11\linewidth]{Figure/2K/RCAN-ClassSR.png} 
         & \includegraphics[width=0.11\linewidth,height=0.11\linewidth]{Figure/2K/RCAN.png}
         & \includegraphics[width=0.11\linewidth,height=0.11\linewidth]{Figure/2K/IMDN.png} 
         & \includegraphics[width=0.11\linewidth,height=0.11\linewidth]{Figure/2K/OSR.png} 
         \\
         & HR & SRResNet-\emph{O}~\cite{SRGAN} & RCAN-\emph{O}~\cite{RCAN} & IMDN-\emph{O}~\cite{IMDN} & \textbf{\algname{}}-\emph{O} \\
         % & &  16.69/5.20G & 17.26/32.60G & 17.26/729M & 18.99/1.96G \\
         & \includegraphics[width=0.11\linewidth,height=0.11\linewidth]{Figure/2K/LR.png} 
         & \includegraphics[width=0.11\linewidth,height=0.11\linewidth]{Figure/2K/RCAN-ClassSR.png} 
         & \includegraphics[width=0.11\linewidth,height=0.11\linewidth]{Figure/2K/RCAN-ClassSR.png}
         & \includegraphics[width=0.11\linewidth,height=0.11\linewidth]{Figure/2K/SwinIR.png} 
         & \includegraphics[width=0.11\linewidth,height=0.11\linewidth]{Figure/2K/OSR05.png} 
         \\
          {\emph{1261} from Test2K} &{LR} & SRResNet-\emph{ClassSR} & RCAN-\emph{ClassSR} & SwinIR-L-\emph{O}~\cite{SwinIR} & \textbf{\algname{}} \\
    \end{tabular}
    \caption{Visual comparison of \algname{} with other methods for $\times$4 task on Test2K and Test4K dataset.}
    \label{fig:Test4K2}
\end{figure*}

\subsection{Lightweight SR}
In~\cref{tab:4} and \cref{fig:3}, we supply the quantitative and qualitative results of CAMixerSR with varied $\gamma$ on the Lightweight SR task. Different from \cref{sec:1}, the CAMixer with $\gamma=0.25$ encounters more extensive PSNR drops (0.06-0.14dB) on benchmark datasets. Moreover, we train our CAMixerSR with a large-scale training set, DF2K~\cite{EDSR} to explore and exploit the maximum representation capability. Similar to previous work~\cite{SwinIR}, using DF2K significantly improves the restoration quality for the baseline model ($\gamma=1.0$). In detail, the PSNR increases by 0.22dB on Manga109~\cite{manga109}. More importantly, for models trained with large-scale sets, reducing the attention area ($\gamma$) can also maintain remarkable performance as using small-scale sets. In conclusion, improving the training schedule would not affect the CAMixer, showing its generality and robustness.

% \begin{figure*}
%     \centering
%     \scriptsize
%     \tabcolsep=2pt
% \begin{tabular}{c}
% \includegraphics[width=0.7\linewidth]{Figure/360/004_OSR_x2.png}\\
% \includegraphics[width=0.7\linewidth]{Figure/360/062_OSR_x4_0.5.png}\\
% \includegraphics[width=0.7\linewidth]{Figure/360/095_OSR_x4_0.5.png}
% \end{tabular}
%     \caption{Visual comparison of \algname{} with other methods for $\times$4 task on SUN 360 dataset.}
%     \label{fig:360}
% \end{figure*}
